# Supplementary material for: Maximizing the number of q-colorings
Source: arXiv:0811.2625 ancillary file (2009-09-25)

$$\text{OPT}[q] := -2 \sqrt{\text{Log}\left[\frac{q}{q-1}\right] \text{Log}[q]}$$

```

(*TESTING q=3*)(*For partition:3=1+1+1*)
ans := N[Maximize[{3 x1 Log[1/3], (3 x1)^2 - (3 x1^2) ≥ 2 && x1 ≥ 0}, {x1}]]
{N[ans][[1]], N[OPT[3]], N[ans][[1]] < N[OPT[3]] - 0.1}
(*For partition:3=1+2*)
(*We already know from one of our lemmas that (for all q≥3)
  if the partition is this,
then the maximum is uniquely achieved at our solution.*)
(*For partition:3=3*)
(*This is the trivial partition,
which we don't need to worry about.*)
(*TESTING q=4*)
(*For partition:4=1+1+1+1*)
ans := N[Maximize[{4 x1 Log[1/4], (4 x1)^2 - (4 x1^2) ≥ 2 && x1 ≥ 0}, {x1}]]
{N[ans][[1]], N[OPT[4]], N[ans][[1]] < N[OPT[4]] - 0.1}
(*For partition:4=1+1+2*)
ans :=
  N[Maximize[{2 x1 Log[1/4] + x2 Log[2/4],
    (2 x1 + x2)^2 - (2 x1^2 + x2^2) ≥ 2 && x1 ≥ 0 && x2 ≥ 0}, {x1, x2}]]
{N[ans][[1]], N[OPT[4]], N[ans][[1]] < N[OPT[4]] - 0.1}
(*For partition:4=1+3*)
(*We already know from one of our lemmas that (for all q≥3)
  if the partition is this,
then the maximum is uniquely achieved at our solution.*)

```

```

(*For partition:4=2+2*)
ans := N[Maximize[{2 x2 Log[2 / 4], (2 x2)^2 - (2 x2^2) ≥ 2 && x2 ≥ 0}, {x2}]]
{N[ans][[1]], N[OPT[4]], N[ans][[1]] < N[OPT[4]] - 0.1}
(*For partition:4=4*)
(*This is the trivial partition,
which we don't need to worry about.*)
(*TESTING q=5*)
(*For partition:5=1+1+1+1+1*)
ans := N[Maximize[{5 x1 Log[1 / 5], (5 x1)^2 - (5 x1^2) ≥ 2 && x1 ≥ 0}, {x1}]]
{N[ans][[1]], N[OPT[5]], N[ans][[1]] < N[OPT[5]] - 0.1}
(*For partition:5=1+1+1+2*)
ans :=
  N[Maximize[{3 x1 Log[1 / 5] + x2 Log[2 / 5],
    (3 x1 + x2)^2 - (3 x1^2 + x2^2) ≥ 2 && x1 ≥ 0 && x2 ≥ 0}, {x1, x2}]]
{N[ans][[1]], N[OPT[5]], N[ans][[1]] < N[OPT[5]] - 0.1}
(*For partition:5=1+1+3*)
ans :=
  N[Maximize[{2 x1 Log[1 / 5] + x3 Log[3 / 5],
    (2 x1 + x3)^2 - (2 x1^2 + x3^2) ≥ 2 && x1 ≥ 0 && x3 ≥ 0}, {x1, x3}]]
{N[ans][[1]], N[OPT[5]], N[ans][[1]] < N[OPT[5]] - 0.1}
(*For partition:5=1+2+2*)
ans :=
  N[Maximize[{x1 Log[1 / 5] + 2 x2 Log[2 / 5],
    (x1 + 2 x2)^2 - (x1^2 + 2 x2^2) ≥ 2 && x1 ≥ 0 && x2 ≥ 0}, {x1, x2}]]
{N[ans][[1]], N[OPT[5]], N[ans][[1]] < N[OPT[5]] - 0.1}
(*For partition:5=1+4*)
(*We already know from one of our lemmas that (for all q≥3)

```

```

if the partition is this,
then the maximum is uniquely achieved at our solution.*)
(*For partition:5=2+3*)
ans :=
N[Maximize[{x2 Log[2 / 5] + x3 Log[3 / 5],
  (x2 + x3)^2 - (x2^2 + x3^2) ≥ 2 && x2 ≥ 0 && x3 ≥ 0}, {x2, x3}]]
{N[ans][[1]], N[OPT[5]], N[ans][[1]] < N[OPT[5]] - 0.1}
(*For partition:5=5*)
(*This is the trivial partition,
which we don't need to worry about.*)
(*TESTING q=6*)
(*For partition:6=1+1+1+1+1+1*)
ans := N[Maximize[{6 x1 Log[1 / 6], (6 x1)^2 - (6 x1^2) ≥ 2 && x1 ≥ 0}, {x1}]]
{N[ans][[1]], N[OPT[6]], N[ans][[1]] < N[OPT[6]] - 0.1}
(*For partition:6=1+1+1+1+2*)
ans :=
N[Maximize[{4 x1 Log[1 / 6] + x2 Log[2 / 6],
  (4 x1 + x2)^2 - (4 x1^2 + x2^2) ≥ 2 && x1 ≥ 0 && x2 ≥ 0}, {x1, x2}]]
{N[ans][[1]], N[OPT[6]], N[ans][[1]] < N[OPT[6]] - 0.1}
(*For partition:6=1+1+1+3*)
ans :=
N[Maximize[{3 x1 Log[1 / 6] + x3 Log[3 / 6],
  (3 x1 + x3)^2 - (3 x1^2 + x3^2) ≥ 2 && x1 ≥ 0 && x3 ≥ 0}, {x1, x3}]]
{N[ans][[1]], N[OPT[6]], N[ans][[1]] < N[OPT[6]] - 0.1}
(*For partition:6=1+1+2+2*)
ans :=
N[Maximize[{2 x1 Log[1 / 6] + 2 x2 Log[2 / 6],

```

```

      (2 x1 + 2 x2) ^ 2 - (2 x1 ^ 2 + 2 x2 ^ 2) ≥ 2 && x1 ≥ 0 && x2 ≥ 0}, {x1, x2}]]
{N[ans][[1]], N[OPT[6]], N[ans][[1]] < N[OPT[6]] - 0.1}
(*For partition:6=1+1+4*)
ans :=
N[Maximize[{2 x1 Log[1 / 6] + x4 Log[4 / 6],
      (2 x1 + x4) ^ 2 - (2 x1 ^ 2 + x4 ^ 2) ≥ 2 && x1 ≥ 0 && x4 ≥ 0}, {x1, x4}]]
{N[ans][[1]], N[OPT[6]], N[ans][[1]] < N[OPT[6]] - 0.1}
(*For partition:6=1+2+3*)
ans :=
N[Maximize[{x1 Log[1 / 6] + x2 Log[2 / 6] + x3 Log[3 / 6],
      (x1 + x2 + x3) ^ 2 - (x1 ^ 2 + x2 ^ 2 + x3 ^ 2) ≥ 2 && x1 ≥ 0 && x2 ≥ 0 && x3 ≥ 0},
      {x1, x2, x3}]]
{N[ans][[1]], N[OPT[6]], N[ans][[1]] < N[OPT[6]] - 0.1}
(*For partition:6=1+5*)
(*We already know from one of our lemmas that (for all q≥3)
if the partition is this,
then the maximum is uniquely achieved at our solution.*)
(*For partition:6=2+2+2*)
ans := N[Maximize[{3 x2 Log[2 / 6], (3 x2) ^ 2 - (3 x2 ^ 2) ≥ 2 && x2 ≥ 0}, {x2}]]
{N[ans][[1]], N[OPT[6]], N[ans][[1]] < N[OPT[6]] - 0.1}
(*For partition:6=2+4*)
ans :=
N[Maximize[{x2 Log[2 / 6] + x4 Log[4 / 6],
      (x2 + x4) ^ 2 - (x2 ^ 2 + x4 ^ 2) ≥ 2 && x2 ≥ 0 && x4 ≥ 0}, {x2, x4}]]
{N[ans][[1]], N[OPT[6]], N[ans][[1]] < N[OPT[6]] - 0.1}
(*For partition:6=3+3*)
ans := N[Maximize[{2 x3 Log[3 / 6], (2 x3) ^ 2 - (2 x3 ^ 2) ≥ 2 && x3 ≥ 0}, {x3}]]

```

```

{N[ans][[1]], N[OPT[6]], N[ans][[1]] < N[OPT[6]] - 0.1}
(*For partition:6=6*)
(*This is the trivial partition,
which we don't need to worry about.*)
(*TESTING q=7*)
(*For partition:7=1+1+1+1+1+1+1*)
ans := N[Maximize[{7 x1 Log[1 / 7], (7 x1)^2 - (7 x1^2) ≥ 2 && x1 ≥ 0}, {x1}]]
{N[ans][[1]], N[OPT[7]], N[ans][[1]] < N[OPT[7]] - 0.1}
(*For partition:7=1+1+1+1+1+2*)
ans :=
  N[Maximize[{5 x1 Log[1 / 7] + x2 Log[2 / 7],
    (5 x1 + x2)^2 - (5 x1^2 + x2^2) ≥ 2 && x1 ≥ 0 && x2 ≥ 0}, {x1, x2}]]
{N[ans][[1]], N[OPT[7]], N[ans][[1]] < N[OPT[7]] - 0.1}
(*For partition:7=1+1+1+1+3*)
ans :=
  N[Maximize[{4 x1 Log[1 / 7] + x3 Log[3 / 7],
    (4 x1 + x3)^2 - (4 x1^2 + x3^2) ≥ 2 && x1 ≥ 0 && x3 ≥ 0}, {x1, x3}]]
{N[ans][[1]], N[OPT[7]], N[ans][[1]] < N[OPT[7]] - 0.1}
(*For partition:7=1+1+1+2+2*)
ans :=
  N[Maximize[{3 x1 Log[1 / 7] + 2 x2 Log[2 / 7],
    (3 x1 + 2 x2)^2 - (3 x1^2 + 2 x2^2) ≥ 2 && x1 ≥ 0 && x2 ≥ 0}, {x1, x2}]]
{N[ans][[1]], N[OPT[7]], N[ans][[1]] < N[OPT[7]] - 0.1}
(*For partition:7=1+1+1+4*)
ans :=
  N[Maximize[{3 x1 Log[1 / 7] + x4 Log[4 / 7],
    (3 x1 + x4)^2 - (3 x1^2 + x4^2) ≥ 2 && x1 ≥ 0 && x4 ≥ 0}, {x1, x4}]]

```

```

{N[ans][[1]], N[OPT[7]], N[ans][[1]] < N[OPT[7]] - 0.1}
(*For partition:7=1+1+2+3*)
ans :=
N[Maximize[{2 x1 Log[1/7] + x2 Log[2/7] + x3 Log[3/7],
(2 x1 + x2 + x3)^2 - (2 x1^2 + x2^2 + x3^2) ≥ 2 && x1 ≥ 0 && x2 ≥ 0 && x3 ≥ 0},
{x1, x2, x3}]]
{N[ans][[1]], N[OPT[7]], N[ans][[1]] < N[OPT[7]] - 0.1}
(*For partition:7=1+1+5*)
ans :=
N[Maximize[{2 x1 Log[1/7] + x5 Log[5/7],
(2 x1 + x5)^2 - (2 x1^2 + x5^2) ≥ 2 && x1 ≥ 0 && x5 ≥ 0}, {x1, x5}]]
{N[ans][[1]], N[OPT[7]], N[ans][[1]] < N[OPT[7]] - 0.1}
(*For partition:7=1+2+2+2*)
ans :=
N[Maximize[{x1 Log[1/7] + 3 x2 Log[2/7],
(x1 + 3 x2)^2 - (x1^2 + 3 x2^2) ≥ 2 && x1 ≥ 0 && x2 ≥ 0}, {x1, x2}]]
{N[ans][[1]], N[OPT[7]], N[ans][[1]] < N[OPT[7]] - 0.1}
(*For partition:7=1+2+4*)
ans :=
N[Maximize[{x1 Log[1/7] + x2 Log[2/7] + x4 Log[4/7],
(x1 + x2 + x4)^2 - (x1^2 + x2^2 + x4^2) ≥ 2 && x1 ≥ 0 && x2 ≥ 0 && x4 ≥ 0},
{x1, x2, x4}]]
{N[ans][[1]], N[OPT[7]], N[ans][[1]] < N[OPT[7]] - 0.1}
(*For partition:7=1+3+3*)
ans :=
N[Maximize[{x1 Log[1/7] + 2 x3 Log[3/7],
(x1 + 2 x3)^2 - (x1^2 + 2 x3^2) ≥ 2 && x1 ≥ 0 && x3 ≥ 0}, {x1, x3}]]

```

```

{N[ans][[1]], N[OPT[7]], N[ans][[1]] < N[OPT[7]] - 0.1}
(*For partition:7=1+6*)
(*We already know from one of our lemmas that (for all q≥3)
  if the partition is this,
then the maximum is uniquely achieved at our solution.*)
(*For partition:7=2+2+3*)
ans :=
N[Maximize[{2 x2 Log[2 / 7] + x3 Log[3 / 7],
  (2 x2 + x3)^2 - (2 x2^2 + x3^2) ≥ 2 && x2 ≥ 0 && x3 ≥ 0}, {x2, x3}]]
{N[ans][[1]], N[OPT[7]], N[ans][[1]] < N[OPT[7]] - 0.1}
(*For partition:7=2+5*)
ans :=
N[Maximize[{x2 Log[2 / 7] + x5 Log[5 / 7],
  (x2 + x5)^2 - (x2^2 + x5^2) ≥ 2 && x2 ≥ 0 && x5 ≥ 0}, {x2, x5}]]
{N[ans][[1]], N[OPT[7]], N[ans][[1]] < N[OPT[7]] - 0.1}
(*For partition:7=3+4*)
ans :=
N[Maximize[{x3 Log[3 / 7] + x4 Log[4 / 7],
  (x3 + x4)^2 - (x3^2 + x4^2) ≥ 2 && x3 ≥ 0 && x4 ≥ 0}, {x3, x4}]]
{N[ans][[1]], N[OPT[7]], N[ans][[1]] < N[OPT[7]] - 0.1}
(*For partition:7=7*)
(*This is the trivial partition,
which we don't need to worry about.*)
(*TESTING q=8*)
(*For partition:8=1+1+1+1+1+1+1+1*)
ans := N[Maximize[{8 x1 Log[1 / 8], (8 x1)^2 - (8 x1^2) ≥ 2 && x1 ≥ 0}, {x1}]]
{N[ans][[1]], N[OPT[8]], N[ans][[1]] < N[OPT[8]] - 0.1}

```

```

(*For partition:8=1+1+1+1+1+1+2*)
ans :=
N[Maximize[{6 x1 Log[1 / 8] + x2 Log[2 / 8],
(6 x1 + x2)^2 - (6 x1^2 + x2^2) ≥ 2 && x1 ≥ 0 && x2 ≥ 0}, {x1, x2}]]
{N[ans][[1]], N[OPT[8]], N[ans][[1]] < N[OPT[8]] - 0.1}
(*For partition:8=1+1+1+1+1+3*)
ans :=
N[Maximize[{5 x1 Log[1 / 8] + x3 Log[3 / 8],
(5 x1 + x3)^2 - (5 x1^2 + x3^2) ≥ 2 && x1 ≥ 0 && x3 ≥ 0}, {x1, x3}]]
{N[ans][[1]], N[OPT[8]], N[ans][[1]] < N[OPT[8]] - 0.1}
(*For partition:8=1+1+1+1+2+2*)
ans :=
N[Maximize[{4 x1 Log[1 / 8] + 2 x2 Log[2 / 8],
(4 x1 + 2 x2)^2 - (4 x1^2 + 2 x2^2) ≥ 2 && x1 ≥ 0 && x2 ≥ 0}, {x1, x2}]]
{N[ans][[1]], N[OPT[8]], N[ans][[1]] < N[OPT[8]] - 0.1}
(*For partition:8=1+1+1+1+4*)
ans :=
N[Maximize[{4 x1 Log[1 / 8] + x4 Log[4 / 8],
(4 x1 + x4)^2 - (4 x1^2 + x4^2) ≥ 2 && x1 ≥ 0 && x4 ≥ 0}, {x1, x4}]]
{N[ans][[1]], N[OPT[8]], N[ans][[1]] < N[OPT[8]] - 0.1}
(*For partition:8=1+1+1+2+3*)
ans :=
N[Maximize[{3 x1 Log[1 / 8] + x2 Log[2 / 8] + x3 Log[3 / 8],
(3 x1 + x2 + x3)^2 - (3 x1^2 + x2^2 + x3^2) ≥ 2 && x1 ≥ 0 && x2 ≥ 0 && x3 ≥ 0},
{x1, x2, x3}]]
{N[ans][[1]], N[OPT[8]], N[ans][[1]] < N[OPT[8]] - 0.1}
(*For partition:8=1+1+1+5*)

```

```

ans :=
  N[Maximize[{3 x1 Log[1 / 8] + x5 Log[5 / 8],
    (3 x1 + x5)^2 - (3 x1^2 + x5^2) ≥ 2 && x1 ≥ 0 && x5 ≥ 0}, {x1, x5}]]
{N[ans][[1]], N[OPT[8]], N[ans][[1]] < N[OPT[8]] - 0.1}
(*For partition:8=1+1+2+2+2*)
ans :=
  N[Maximize[{2 x1 Log[1 / 8] + 3 x2 Log[2 / 8],
    (2 x1 + 3 x2)^2 - (2 x1^2 + 3 x2^2) ≥ 2 && x1 ≥ 0 && x2 ≥ 0}, {x1, x2}]]
{N[ans][[1]], N[OPT[8]], N[ans][[1]] < N[OPT[8]] - 0.1}
(*For partition:8=1+1+2+4*)
ans :=
  N[Maximize[{2 x1 Log[1 / 8] + x2 Log[2 / 8] + x4 Log[4 / 8],
    (2 x1 + x2 + x4)^2 - (2 x1^2 + x2^2 + x4^2) ≥ 2 && x1 ≥ 0 && x2 ≥ 0 && x4 ≥ 0},
    {x1, x2, x4}]]
{N[ans][[1]], N[OPT[8]], N[ans][[1]] < N[OPT[8]] - 0.1}
(*For partition:8=1+1+3+3*)
ans :=
  N[Maximize[{2 x1 Log[1 / 8] + 2 x3 Log[3 / 8],
    (2 x1 + 2 x3)^2 - (2 x1^2 + 2 x3^2) ≥ 2 && x1 ≥ 0 && x3 ≥ 0}, {x1, x3}]]
{N[ans][[1]], N[OPT[8]], N[ans][[1]] < N[OPT[8]] - 0.1}
(*For partition:8=1+1+6*)
ans :=
  N[Maximize[{2 x1 Log[1 / 8] + x6 Log[6 / 8],
    (2 x1 + x6)^2 - (2 x1^2 + x6^2) ≥ 2 && x1 ≥ 0 && x6 ≥ 0}, {x1, x6}]]
{N[ans][[1]], N[OPT[8]], N[ans][[1]] < N[OPT[8]] - 0.1}
(*For partition:8=1+2+2+3*)
ans :=

```

```

N[Maximize[{x1 Log[1/8] + 2 x2 Log[2/8] + x3 Log[3/8],
  (x1 + 2 x2 + x3)^2 - (x1^2 + 2 x2^2 + x3^2) ≥ 2 && x1 ≥ 0 && x2 ≥ 0 && x3 ≥ 0},
  {x1, x2, x3}]]
{N[ans][[1]], N[OPT[8]], N[ans][[1]] < N[OPT[8]] - 0.1}
(*For partition:8=1+2+5*)
ans :=
N[Maximize[{x1 Log[1/8] + x2 Log[2/8] + x5 Log[5/8],
  (x1 + x2 + x5)^2 - (x1^2 + x2^2 + x5^2) ≥ 2 && x1 ≥ 0 && x2 ≥ 0 && x5 ≥ 0},
  {x1, x2, x5}]]
{N[ans][[1]], N[OPT[8]], N[ans][[1]] < N[OPT[8]] - 0.1}
(*For partition:8=1+3+4*)
ans :=
N[Maximize[{x1 Log[1/8] + x3 Log[3/8] + x4 Log[4/8],
  (x1 + x3 + x4)^2 - (x1^2 + x3^2 + x4^2) ≥ 2 && x1 ≥ 0 && x3 ≥ 0 && x4 ≥ 0},
  {x1, x3, x4}]]
{N[ans][[1]], N[OPT[8]], N[ans][[1]] < N[OPT[8]] - 0.1}
(*For partition:8=1+7*)
(*We already know from one of our lemmas that (for all q≥3)
  if the partition is this,
  then the maximum is uniquely achieved at our solution.*)
(*For partition:8=2+2+2+2*)
ans := N[Maximize[{4 x2 Log[2/8], (4 x2)^2 - (4 x2^2) ≥ 2 && x2 ≥ 0}, {x2}]]
{N[ans][[1]], N[OPT[8]], N[ans][[1]] < N[OPT[8]] - 0.1}
(*For partition:8=2+2+4*)
ans :=
N[Maximize[{2 x2 Log[2/8] + x4 Log[4/8],
  (2 x2 + x4)^2 - (2 x2^2 + x4^2) ≥ 2 && x2 ≥ 0 && x4 ≥ 0}, {x2, x4}]]

```

```

{N[ans][[1]], N[OPT[8]], N[ans][[1]] < N[OPT[8]] - 0.1}
(*For partition:8=2+3+3*)
ans :=
N[Maximize[{x2 Log[2/8] + 2 x3 Log[3/8],
  (x2 + 2 x3)^2 - (x2^2 + 2 x3^2) ≥ 2 && x2 ≥ 0 && x3 ≥ 0}, {x2, x3}]]
{N[ans][[1]], N[OPT[8]], N[ans][[1]] < N[OPT[8]] - 0.1}
(*For partition:8=2+6*)
ans :=
N[Maximize[{x2 Log[2/8] + x6 Log[6/8],
  (x2 + x6)^2 - (x2^2 + x6^2) ≥ 2 && x2 ≥ 0 && x6 ≥ 0}, {x2, x6}]]
{N[ans][[1]], N[OPT[8]], N[ans][[1]] < N[OPT[8]] - 0.1}
(*For partition:8=3+5*)
ans :=
N[Maximize[{x3 Log[3/8] + x5 Log[5/8],
  (x3 + x5)^2 - (x3^2 + x5^2) ≥ 2 && x3 ≥ 0 && x5 ≥ 0}, {x3, x5}]]
{N[ans][[1]], N[OPT[8]], N[ans][[1]] < N[OPT[8]] - 0.1}
(*For partition:8=4+4*)
ans := N[Maximize[{2 x4 Log[4/8], (2 x4)^2 - (2 x4^2) ≥ 2 && x4 ≥ 0}, {x4}]]
{N[ans][[1]], N[OPT[8]], N[ans][[1]] < N[OPT[8]] - 0.1}
(*For partition:8=8*)
(*This is the trivial partition,
which we don't need to worry about.*)

{-1.90285, -1.33484, True}

{-2.26381, -1.26303, True}

```

```
{-1.8339, -1.26303, True}
```

```
{-1.38629, -1.26303, True}
```

```
{-2.54474, -1.19856, True}
```

```
{-2.18618, -1.19856, True}
```

```
{-1.74001, -1.19856, True}
```

```
{-1.81895, -1.19856, True}
```

```
{-1.36831, -1.19856, True}
```

```
{-2.77578, -1.14311, True}
```

```
{-2.46239, -1.14311, True}
```

```
{-2.08019, -1.14311, True}
```

```
{-2.14676, -1.14311, True}
```

```
{-1.65577, -1.14311, True}
```

```
Maximize::ztest: Unable to decide whether numeric  
quantities {Log[2] + Log[3] - Log[6]} are equal to zero. Assuming they are. >>
```

```
Maximize::ztest: Unable to decide whether numeric  
quantities {Log[2] + Log[3] - Log[6]} are equal to zero. Assuming they are. >>
```

```
{-1.74528, -1.14311, True}
```

```
{-1.90285, -1.14311, True}
```

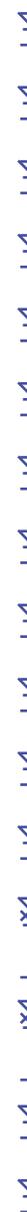

{-1.33484, -1.14311, True}

{-1.38629, -1.14311, True}

{-2.97243, -1.09538, True}

{-2.69072, -1.09538, True}

{-2.34908, -1.09538, True}

{-2.40996, -1.09538, True}

{-1.98451, -1.09538, True}

{-2.05284, -1.09538, True}

{-1.58296, -1.09538, True}

{-2.16985, -1.09538, True}

{-1.67459, -1.09538, True}

{-1.6946, -1.09538, True}

{-1.87828, -1.09538, True}

{-1.29849, -1.09538, True}

{-1.37719, -1.09538, True}

{-3.14382, -1.05389, True}

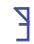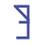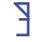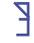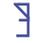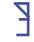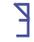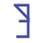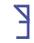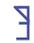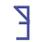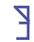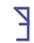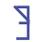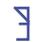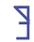

{-2.8858, -1.05389, True}

{-2.57275, -1.05389, True}

{-2.63031, -1.05389, True}

{-2.24605, -1.05389, True}

{-2.30537, -1.05389, True}

{-1.90127, -1.05389, True}

Maximize::ztest: Unable to decide whether numeric

quantities  $\left\{ \frac{1}{2} (3 \text{Log}[4] - 2 \text{Log}[8]) \right\}$  are equal to zero. Assuming they are. >>

Maximize::ztest: Unable to decide whether numeric

quantities  $\left\{ \frac{1}{2} (3 \text{Log}[4] - 2 \text{Log}[8]) \right\}$  are equal to zero. Assuming they are. >>

{-2.40113, -1.05389, True}

Maximize::ztest: Unable to decide whether numeric quantities

$\{2 \text{Log}[2] - \text{Log}[4], \text{Log}[2] + \text{Log}[4] - \text{Log}[8]\}$  are equal to zero. Assuming they are. >>

Maximize::ztest: Unable to decide whether numeric quantities

$\{2 \text{Log}[2] - \text{Log}[4], \text{Log}[2] + \text{Log}[4] - \text{Log}[8]\}$  are equal to zero. Assuming they are. >>

{-1.96052, -1.05389, True}

{-1.96166, -1.05389, True}

{-1.51991, -1.05389, True}

{-2.11586, -1.05389, True}

{-1.61439, -1.05389, True}

{-1.64907, -1.05389, True}

{-2.26381, -1.05389, True}

{-1.8339, -1.05389, True}

{-1.87538, -1.05389, True}

{-1.26303, -1.05389, True}

{-1.35793, -1.05389, True}

{-1.38629, -1.05389, True}

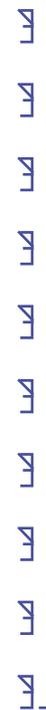

Supplement: Supplementary file 1 [file solve-sparse-opt-check-small.pdf]
